# Supplementary material for: PP-SAM: Perturbed Prompts for Robust Adaptation of Segment Anything Model for Polyp Segmentation
Source: arXiv:2405.16740 source file (2024-05-27)
Supplement: Supplementary file 1 [file X_suppl.tex]

\clearpage
\setcounter{page}{1}
\maketitlesupplementary

\section{Experimental Details}
\label{asec:more_experiments}
This section extends our \cref{sec:experiments} in the original paper by describing the datasets and evaluation metrics, followed by additional experimental results.

\begin{table*}[]
\begin{center}
    {%\small{
\begin{adjustbox}{width=0.98\textwidth}
{\begin{tabular}{lc|rrr|rrrrrrrrr}
\toprule
\multirow{2}{*}{Architectures} & \multirow{2}{*}{Pretrain} & \multicolumn{3}{c|}{Average}                                                                                     & \multicolumn{1}{l}{\multirow{2}{*}{Aorta}} & \multicolumn{1}{l}{\multirow{2}{*}{GB}} & \multicolumn{1}{l}{\multirow{2}{*}{KL}} & \multicolumn{1}{l}{\multirow{2}{*}{KR}} & \multicolumn{1}{l}{\multirow{2}{*}{Liver}} & \multicolumn{1}{l}{\multirow{2}{*}{PC}} & \multicolumn{1}{l}{\multirow{2}{*}{SP}} & \multicolumn{1}{l}{\multirow{2}{*}{SM}} \\
                              & & \multicolumn{1}{l}{DICE$\uparrow$} & \multicolumn{1}{l}{HD95$\downarrow$} & \multicolumn{1}{l|}{mIoU$\uparrow$} & \multicolumn{1}{l}{} & \multicolumn{1}{l}{} & \multicolumn{1}{l}{} & \multicolumn{1}{l}{} & \multicolumn{1}{l}{} & \multicolumn{1}{l}{} & \multicolumn{1}{l}{} & \multicolumn{1}{l}{}      \\
\midrule %+0.2
PVT-EMCAD-B0     & No     & 75.25 &   23.85  &  64.34 &   80.19 &  62.07  &   80.19  &   76.12 &  92.80  &   49.25 &   89.30 & 71.71 \\
PVT-EMCAD-B0      & Yes     & 81.05 &   17.47  &  71.23   &   84.26   &  68.25  & 84.03  &   82.07 &  94.20 &   63.12   &   90.80   & 82.05 \\
\midrule
PVT-EMCAD-B2         & No        & 79.57   & 17.93   & 69.27  &  84.83   &    69.86  & 82.13   & 76.63  & 94.38   & 62.40  & \textbf{91.20}   & 75.10
\\
PVT-EMCAD-B2      & Yes   & \textbf{83.16}  & \textbf{12.96}   & \textbf{74.73}  &  \textbf{87.96}  &    \textbf{71.10}  & \textbf{86.01} & \textbf{84.68} & \textbf{95.30} & \textbf{66.20}  & 90.51 & \textbf{83.56} \\
\bottomrule
\end{tabular}}
\end{adjustbox}
}%}
\end{center}
\vspace{-0.4cm}
\caption{Effect of transfer learning from ImageNet pre-trained weights on Synapse multi-organ dataset. $\uparrow$ ($\downarrow$) denotes the higher (lower) the better. All results are averaged over five runs. Best results are in bold.}
\vspace{-0.1cm}
\label{tab:transfer_learing}
\end{table*}

\subsection{Datasets}
\label{assec:dataset_metrics}
\vspace{-.1cm}
To evaluate the performance of our EMCAD decoder, we carry out experimental analyses across 12 datasets that belong to six standard medical image segmentation tasks, as described next. %We present the description of abdomen organ, cardiac organ, polyp, Skin lesion, cell, and breast cancer segmentation datasets below.%, and retinal vessel segmentation datasets are described in supplementary materials (Section A).

\noindent \textbf{Polyp segmentation:} We use five polyp segmentation datasets: Kvasir \cite{jha2020kvasir} (1,000 images), ClinicDB \cite{bernal2015wm} (612 images), ColonDB \cite{vazquez2017benchmark}
(379 images), ETIS \cite{vazquez2017benchmark} (196 images), and BKAI \cite{ngoc2021neounet} (1,000 images). These datasets contain images from different imaging centers/clinics, having greater diversity in image nature as well as size and shape of polyps. 

\noindent \textbf{Abdomen organ segmentation:} We use the Synapse multi-organ dataset\footnote{\href{https://www.synapse.org/\#!Synapse:syn3193805/wiki/217789}{https://www.synapse.org/\#!Synapse:syn3193805/wiki/217789 }} for abdomen organ segmentation. This dataset contains 30 abdominal CT scans which have 3,779 axial contrast-enhanced slices. Each CT scan has 85-198 slices of $512 \times 512$ pixels.
Following TransUNet \cite{chen2021transunet}, we use the same 18 scans for training (2,212 axial slices) and 12 scans for validation. We segment only eight abdominal organs, namely aorta, gallbladder (GB), left kidney (KL), right kidney (KR), liver, pancreas (PC), spleen (SP), and stomach (SM). 

\noindent \textbf{Cardiac organ segmentation:} We use ACDC dataset\footnote{\href{https://www.creatis.insa-lyon.fr/Challenge/acdc/}{https://www.creatis.insa-lyon.fr/Challenge/acdc/}} for cardiac organ segmentation. It contains 100 cardiac MRI scans having three sub-organs, namely right ventricle (RV), myocardium (Myo), and left ventricle (LV). Following TransUNet \cite{chen2021transunet}, we use 70 cases (1,930 axial slices) for training, 10 for validation, and 20 for testing. 

\noindent \textbf{Skin lesion segmentation:} We use ISIC17 \cite{codella2018skin} (2,000 training, 150 validation, and 600 testing images) and ISIC18 \cite{codella2019skin} (2,594 images) for skin lesion segmentation. 

\noindent \textbf{Breast cancer segmentation:} We use BUSI \cite{al2020dataset} dataset for breast cancer segmentation. Following \cite{valanarasu2022unext}, we use 647 (437 benign and 210 malignant) images from this dataset. 

\noindent \textbf{Cell nuclei/structure segmentation:} We use the DSB18 \cite{caicedo2019nucleus} (670 images) and EM \cite{cardona2010integrated} (30 images) datasets of biological imaging for cell nuclei/structure segmentation. 

We use a train-val-test split of 80:10:10 in ClinicDB, Kvasir, ColonDB, ETIS, BKAI, ISIC18, DSB18, EM, and BUSI datasets. For ISIC17, we use the official train-val-test sets provided by the competition organizer.  
% and MT\_UNet \cite{wang2022mixed}

\subsection{Evaluation metrics} 
\label{assec:eval_metrics}
We use the DICE score to evaluate performance on all the datasets. However, we also use 95\% Hausdorff Distance (HD95) and mIoU as additional evaluation metrics for Synapse multi-organ segmentation. The DICE score $DSC(Y, P)$, $IoU(Y, P)$, and HD95 distance $D_H(Y, P)$ are calculated using Equations \ref{eq:dice}, \ref{eq:iou}, and \ref{eq:95hd}, respectively:
%(95th percentile of the distances between boundary points in $Y$ and $\hat{Y}$) 
\begin{equation}\label{eq:dice}
DSC(Y, P) = \frac{2 \times \lvert Y \cap P \rvert}{\lvert Y \rvert + \lvert P \rvert}\times100
\end{equation}
\begin{equation}\label{eq:iou}
IoU(Y, P) = \frac{\lvert Y \cap P \rvert}{\lvert Y \cup P \rvert}\times100
\end{equation}
\begin{equation}\label{eq:95hd}
\small
D_H(Y, P) = \max \{\max_{y \in Y} \min_{p \in P}d(y, p), \{\max_{p \in P} \min_{y \in Y}d(y, p)\}
%\max\{d_{Y\hat{Y}},d_{\hat{Y}Y}\} = 
\end{equation}
where $Y$ and $P$ are the ground truth and predicted segmentation map, respectively. 

%Therefore, following the experimental scheme of Polyp-PVT \cite{dong2021polyp}, we train and test PVT-CASCADE on the Kavsir-SEG [8] and CVC-ClinicDB [1] benchmark datasets, respectively, to assess the accurate prediction and learning ability of models in the Kavsir-SEG and CVC-ClinicDB test set, respectively. 

\subsection{Additional results} 
\label{assec:ddditional_results}

\subsubsection{Effect of transfer learning from ImageNet pre-trained weights}
\label{asec:transfer_learing}
We conduct experiments on the Synapse multi-organ dataset to show the effect of transfer learning from the ImageNet pre-trained encoder. Table \ref{tab:transfer_learing} below reports the results of these experiments which show that transfer learning from ImageNet pre-trained PVT-v2 encoders significantly boosts the performance. Specifically, for PVT-EMCAD-B0, the DICE, mIoU, and HD95 scores are improved by 5.8\%, 6.89\%, and 6.38, respectively. Likewise, for PVT-EMCAD-B2, the DICE, mIoU, and HD95 scores are improved by 3.57\%, 5.46\%, and 4.97, respectively. We can also conclude that transfer learning has a greater impact on the smaller PVT-EMCAD-B0 model than the larger PVT-EMCAD-B2 model. For individual organs, transfer learning significantly boosts the performance of all organ segmentation, except the Spleen (SP) and Liver.  

%\subsubsection{Results of generalizability experiments}
%\label{asec:generalizability_results}

%\subsubsection{Qualitative results}
%\label{asec:qualitative_results}

\section{Additional Ablation Study}
\label{asec:ablation}
%This section extends \cref{sec:ablation_study} by describing three more ablation studies related to our architectural design and experimental setup. 
This section further elaborates on \cref{sec:ablation_study} by detailing three additional ablation studies related to our architectural design and experimental setup.
%\subsection{Effectiveness of GAG over AG}

\begin{table}[t]
\centering 
    {%\small{
\begin{adjustbox}{width=0.48\textwidth}
{\begin{tabular}{lcrrrr}
\toprule
Architectures & Depth-wise convolutions & \multicolumn{1}{r}{Synapse} & \multicolumn{1}{r}{ClinicDB}\\
\midrule
PVT-EMCAD-B0 & Sequential & 80.92$\pm$0.3 & 94.69$\pm$0.2
\\ PVT-EMCAD-B0 & Parallel  & \textbf{81.05$\pm$0.2} & \textbf{94.72$\pm$0.2} \\
\midrule
PVT-EMCAD-B2 & Sequential  & 83.10$\pm$0.3  & 95.27$\pm$0.3
\\ PVT-EMCAD-B2 &  Parallel  & \textbf{83.16$\pm$0.2}  & \textbf{95.37$\pm$0.2} \\
\bottomrule %\\
\end{tabular}}
\end{adjustbox}

}%}
\vspace{-0.1cm}
\caption{Results of parallel and sequential depth-wise convolution in MSDC on Synapse multi-organ and ClinicDB datasets. All results are averaged over five runs. Best results are in bold.}
\vspace{-0.1cm}
\label{tab:arrangements_parallel_seq}
\end{table}

%\subsection{Attention scores visualization of different components}

\subsection{Parallel vs. sequential depth-wise convolution}
\label{assec:parallel_seq}
We have conducted another set of ablation experiments to decide whether we use multi-scale depth-wise convolutions in parallel or sequential. Table \ref{tab:arrangements_parallel_seq} below presents the results of these experiments which show that there is no significant impact of these arrangements though parallel provides a slightly improved performance (0.03\% to 0.1\%). We also observe higher standard deviations among runs in the case of sequential convolutions. Hence, in all our experiments, we use multi-scale depth-wise convolutions \textit{in parallel}.

\begin{table}[t]
\centering 
    {%\small{
\begin{adjustbox}{width=0.48\textwidth}
{\begin{tabular}{lcrrr}
\toprule
Architectures & Module  & \multicolumn{1}{r}{Params(K)} & \multicolumn{1}{r}{FLOPs(M)} &\multicolumn{1}{r}{Synapse}\\
\midrule
PVT-EMCAD-B0 & AG & 31.62 & 15.91 & 80.92
\\ PVT-EMCAD-B0 & \textbf{LGAG}  & \textbf{5.51} & \textbf{5.24} & \textbf{81.05}\\
\midrule
PVT-EMCAD-B2 & AG  & 124.68  & 61.68 & 83.00
\\ PVT-EMCAD-B2 &  \textbf{LGAG}  & \textbf{11.01}  & \textbf{10.47} & \textbf{83.16} \\
\bottomrule %\\
\end{tabular}}
\end{adjustbox}

}%}
\vspace{-0.2cm}
\caption{LGAG vs. AG (Attention gate) \cite{oktay2018attention} on Synapse multi-organ dataset. The total \#Params and \#FLOPs of three AG/LGAGs in our decoder are reported for an input resolution of $256\times256$. All results are averaged over five runs. Best results are in bold.}
\vspace{-0.1cm}
\label{tab:lgag_vs_ag}
\end{table}

\begin{table}[t]
\centering 
    {%\small{
\begin{adjustbox}{width=0.48\textwidth}
{\begin{tabular}{lrrrrr}
\toprule
Architectures & Resolutions  & \multicolumn{1}{r}{FLOPs(G)} & \multicolumn{1}{r}{DICE}\\ %&
%\midrule
%Parallel MERIT \cite{rahman2023multi} & $256\times256$ & 33.31 &  84.22
%\\ Cascaded MERIT \cite{rahman2023multi} & $256\times256$  & 33.31 &  84.90 \\

\midrule
PVT-EMCAD-B0  & $224\times224$ & 0.64 & 81.05
\\ PVT-EMCAD-B0 & $256\times256$  & 0.84 &  81.89 \\
PVT-EMCAD-B0  & $384\times384$  &  1.89 & 84.42 \\
PVT-EMCAD-B0  & $512\times512$  & 3.36 & 85.11 \\
\midrule
PVT-EMCAD-B2 & $224\times224$  & 4.29  & 83.16
\\
PVT-EMCAD-B2  &  $256\times256$ & 5.60  & 84.17 \\
PVT-EMCAD-B2  &  $384\times384$ &  12.59  & 85.50 \\
PVT-EMCAD-B2  &  $512\times512$ &  22.39 & 86.25 \\
\bottomrule %\\
\end{tabular}}
\end{adjustbox}

}%}
\vspace{-0.2cm}
\caption{Effect of input resolutions on Synapse multi-organ dataset. All results are averaged over five runs.}
\vspace{-0.2cm}
\label{tab:effect_input_resolutions}
\end{table}

\subsection{Effectiveness of our large-kernel grouped attention gate (LGAG) over attention gate (AG)}
\label{assec:lgag_vs_ag}
Table \ref{tab:lgag_vs_ag} presents experimental results of EMCAD with original AG \cite{oktay2018attention} and our LGAG. We can conclude that our LGAG achieves better DICE scores with significant reductions in \#Params (82.57\% for PVT-EMCAD-B0 and 91.17\% for PVT-EMCAD-B2) and \#FLOPs (67.06\% for PVT-EMCAD-B0 and 83.03\% for PVT-EMCAD-B2) than AG. The reduction in \#Params and \#FLOPs is bigger for the larger models. Therefore, our LGAG demonstrates improved scalability with models that have a greater number of channels, yielding enhanced DICE scores.   
%Therefore, our LGAG scales better with the models that have a larger number of channels, yielding enhanced DICE scores. 

\subsection{Effect of input resolutions}
\label{asec:effect_input_resolutions}
Table \ref{tab:effect_input_resolutions} presents the results of our PVT-EMCAD-B0 and PVT-EMCAD-B2 architectures with different input resolutions. From this table, it is evident that the DICE scores improve with the increase in input resolution. However, these improvements in DICE score come with the increment in \#FLOPs. Our PVT-EMCAD-B0 achieves an 85.11\% DICE score with only 3.36G FLOPs when using $512\times512$ inputs. On the other hand, our PVT-EMCAD-B2 achieves the best DICE score (86.25\%) with 22.39G FLOPs when using $512\times512$ inputs. We also observe that our PVT-EMCAD-B2 with 5.60G FLOPs when using $256\times256$ inputs shows a 0.94\% lower DICE score than PVT-EMCAD-B0 with 3.36G FLOPs. Therefore, we can conclude that PVT-EMCAD-B0 is more suitable for larger input resolutions than PVT-EMCAD-B2.   

%We also report the result of the SOTA method, MERIT \cite{rahman2023multi}.  

\section*{Source Code}
\label{asec:source_code}
We will make the source code publicly available with proper documentation upon paper acceptance.
